# Supplementary material for: Learning to Diagnose with LSTM Recurrent Neural Networks
Source: arXiv:1511.03677 source file (2017-03-21)
Supplement: Supplementary file 1 [file diagnosis-appendix-old.tex]

% \begin{figure*}[ht]
\begin{table*}[ht]
\centering
\footnotesize
% \scriptsize
\begin{tabular}{|l|l|l|l|l|l|}
 \hline
 \multicolumn{6}{|c|}{Classifier Performance on Each Diagnostic Code Sorted by AUC} \\
 \hline
  Label & \textbf{AUC} & AUPRC & F1 & Precision & Recall \\
 \hline

Asthma & 0.9439 & 0.7657 & 0.6315 & 0.9230 & 0.48\\ 
Child abuse & 0.9434 & 0.1278 & 0.1 & 0.1111 & 0.0909\\ 
Pulmonary congestion and hypostasis & 0.9386 & 0.0502 & 0.0833 & 0.0476 & 0.3333\\ 
Respiratory syncytial virus & 0.9376 & 0.2047 & 0.2222 & 0.2142 & 0.2307\\ 
Pneumonia due to adenovirus & 0.9355 & 0.0944 & 0.1621 & 0.1034 & 0.375\\ 
Bronchiolitis due to other infectious organism & 0.9293 & 0.2829 & 0.2051 & 0.2352 & 0.1818\\ 
Agranulocytosis & 0.9259 & 0.0637 & 0.1081 & 0.0689 & 0.25\\ 
Acute Pericarditis & 0.9232 & 0.0639 & 0.0952 & 0.0833 & 0.1111\\ 
Extradural hemorrage following injury without open wound & 0.9222 & 0.0682 & 0.1081 & 0.0740 & 0.2\\ 
Biliary atresia & 0.9220 & 0.1967 & 0.0421 & 0.0224 & 0.3333\\ 
Anoxic brain damage & 0.9184 & 0.0789 & 0.1230 & 0.0740 & 0.3636\\ 
Failure & 0.9169 & 0.3042 & 0.4137 & 0.5 & 0.3529\\ 
Defibrination syndrome & 0.9159 & 0.1617 & 0.24 & 0.25 & 0.2307\\ 
Renal transplant status post & 0.9141 & 0.2893 & 0.1818 & 0.1025 & 0.8\\ 
Insufficiency & 0.9121 & 0.3285 & 0.3076 & 0.2352 & 0.4444\\ 
Liver transplant status post & 0.9111 & 0.0392 & 0.0740 & 0.0416 & 0.3333\\ 
Acidosis & 0.9025 & 0.1633 & 0.2857 & 0.4 & 0.2222\\ 
Injury to multiple and unspecified intrathoracic organs %w/out mention of open wound into cavity 
& 0.9010 & 0.1185 & 0.0176 & 0.0089 & 0.8\\ 
Anomalies of the skull and face bone & 0.9009 & 0.3725 & 0.0346 & 0.0177 & 0.7142\\ 
Diabetes mellitus with ketoacidosis & 0.8994 & 0.7817 & 0.7142 & 0.9090 & 0.5882\\ 
Neurofibromatosis & 0.8985 & 0.0498 & 0.0909 & 0.0666 & 0.1428\\ 
Unspecified pleural effusion & 0.8963 & 0.1980 & 0.0869 & 0.05 & 0.3333\\ 
Septic shock & 0.8905 & 0.2792 & 0.3838 & 0.2714 & 0.6551\\ 
Lung contusion without open wound & 0.8862 & 0.0405 & 0.0333 & 0.0196 & 0.1111\\ 
Congenital hereditary muscular dystrophy & 0.8800 & 0.1636 & 0.3333 & 0.2727 & 0.4285\\ 
Werdnig-Hoffman disease & 0.8786 & 0.0671 & 0.0 & 0.0 & 0.0\\ Infantile cerebral palsy & 0.8754 & 0.2176 & 0.2857 & 0.2903 & 0.2812\\ 
Scoliosis & 0.8646 & 0.7055 & 0.6763 & 0.6595 & 0.6940\\ 
Pneumonia due to inhalation of food or vomitus & 0.8622 & 0.0442 & 0.0888 & 0.0606 & 0.1666\\ 
Grand mal status & 0.8600 & 0.2155 & 0.3010 & 0.2333 & 0.4242\\ 
Acute renal failure & 0.8596 & 0.1796 & 0.3043 & 0.2916 & 0.3181\\ 
Benign intracranial hypertension & 0.8517 & 0.1409 & 0.1276 & 0.0833 & 0.2727\\ 
End stage renal disease on dialysis & 0.8514 & 0.4408 & 0.4285 & 0.3333 & 0.6\\ 
Coma & 0.8501 & 0.0843 & 0.0229 & 0.0116 & 0.8888\\ 
Acute pancreatitis & 0.8487 & 0.0898 & 0.0833 & 0.0447 & 0.6\\ 
Mycoplasma pneumoniae & 0.8456 & 0.0842 & 0.1842 & 0.1186 & 0.4117\\ 
Pulmonary hypertension & 0.8433 & 0.1489 & 0.0975 & 0.0547 & 0.4444\\ 
Unspecified disorder of kidney and ureter & 0.8427 & 0.2282 & 0.3333 & 0.28 & 0.4117\\ 
Congenital heart disease & 0.8385 & 0.0581 & 0.1379 & 0.1 & 0.2222\\ 
Chronic respiratory disease arising in the perinatal period & 0.8383 & 0.1387 & 0.2077 & 0.1777 & 0.25\\ 
Neoplasm & 0.8357 & 0.4464 & 0.4866 & 0.4025 & 0.6153\\ 
Hypertension & 0.8326 & 0.0729 & 0.0917 & 0.05 & 0.5555\\ 
Intracranial injury & 0.8324 & 0.2704 & 0.3 & 0.2330 & 0.4210\\ 
Cardiac arrest, outside hospital & 0.8280 & 0.2598 & 0.0421 & 0.0215 & 0.9523\\ 
Acute lymphoid leukemia & 0.8279 & 0.0945 & 0.1470 & 0.0884 & 0.4347\\ 
Cerebral edema & 0.8263 & 0.0764 & 0.015 & 0.0075 & 0.6\\ 
Pneumococcal pneumonia & 0.8249 & 0.0890 & 0.1754 & 0.1351 & 0.25\\ 
Other spontaneous pneumothorax & 0.8236 & 0.0494 & 0.0941 & 0.0540 & 0.3636\\ 
Diabetes insipidus & 0.8225 & 0.0900 & 0.15 & 0.1111 & 0.2307\\ 
Intracranial hemorrhage & 0.8216 & 0.1468 & 0.1470 & 0.0892 & 0.4166\\ 
Cerebral artery occlusion & 0.8139 & 0.0163 & 0.0256 & 0.0134 & 0.2857\\ 

\hline
\end{tabular} \hspace{-0.2in}
% \label{fig:single-label-total-results}
\label{tab:single-label-total-results}
\caption{Results on performance metrics calculated on the $5$ labels with highest F1.}

\end{table*}
% \end{figure*}

% \begin{figure*}[ht]
\begin{table*}[ht]
\centering
\footnotesize
% \scriptsize
\begin{tabular}{|l|l|l|l|l|l|}
 \hline
 \multicolumn{6}{|c|}{(continued) Classifier Performance on Each Diagnostic Code Sorted by AUC} \\
 \hline
  Label & \textbf{AUC} & AUPRC & F1 & Precision & Recall \\
 \hline

Pneumonia & 0.8139 & 0.0876 & 0.1463 & 0.1 & 0.2727\\ 
Injury to unspecifed intra-abdominal organs % w/out mention of open wound into cavity 
& 0.8101 & 0.1986 & 0.0408 & 0.0212 & 0.5\\ 
Septicemia, not otherwise specified & 0.8097 & 0.1589 & 0.1686 & 0.1076 & 0.3888\\ 
Respriatory complications resulting from a procedure & 0.8068 & 0.2027 & 0.2388 & 0.25 & 0.2285\\ 
Cystic fibrosis with pulmonary mainfestations & 0.8059 & 0.1197 & 0.0320 & 0.0164 & 0.6\\ 
Acute respiratory failure & 0.8057 & 0.3235 & 0.4428 & 0.3604 & 0.5740\\ 
Encephalopathy, not otherwise specified & 0.7991 & 0.0410 & 0.1428 & 0.25 & 0.1\\ 
Arteriousvenous malformation of the brain & 0.7984 & 0.1900 & 0.2448 & 0.24 & 0.25\\ 
Apnea & 0.7978 & 0.1033 & 0.1111 & 0.1333 & 0.0952\\ 
Malignant neoplasm & 0.7902 & 0.0274 & 0.0361 & 0.0192 & 0.3\\ 
Disorder of muscle NEC & 0.7894 & 0.1847 & 0.0347 & 0.0178 & 0.6363\\ 
Other shock & 0.7889 & 0.0257 & 0.0545 & 0.03 & 0.3\\ 
Diabetes mellitus & 0.7861 & 0.0775 & 0.1333 & 0.125 & 0.1428\\ 
Motor vehicle accident involving collision %w/ another motor vehicle
& 0.7853 & 0.0864 & 0.1506 & 0.0956 & 0.3548\\ 
Less than 37 weeks gestation & 0.7847 & 0.1304 & 0.1981 & 0.1594 & 0.2619\\ 
Conditions due to anomaly of unspecified circumstance & 0.7823 & 0.2163 & 0.25 & 0.4285 & 0.1764\\ 
Other respiratory symtpom & 0.7814 & 0.2565 & 0.3333 & 0.2807 & 0.4102\\ 
Supraventricular premature beats & 0.7813 & 0.0455 & 0.0952 & 0.0714 & 0.1428\\ 
Anomalies of the skull and face bone & 0.7797 & 0.0617 & 0.1428 & 0.125 & 0.1666\\ 
Cardiac dysrhythmia & 0.7795 & 0.1699 & 0.125 & 0.1428 & 0.1111\\ 
Other diseases of the respiratory system & 0.7792 & 0.1467 & 0.2020 & 0.2127 & 0.1923\\ 
Obesity & 0.7777 & 0.0418 & 0.0661 & 0.0366 & 0.3333\\ 
Hematemesis & 0.7761 & 0.0129 & 0.0191 & 0.0097 & 0.6\\ 
Pneumonitis due to inhalation of food or vomitus & 0.7756 & 0.0222 & 0.0476 & 0.0256 & 0.3333\\ 
Congenital hydrocephalus & 0.7752 & 0.1847 & 0.2432 & 0.3 & 0.2045\\ 
Fracture & 0.7739 & 0.1425 & 0.0740 & 0.0625 & 0.0909\\ 
Other primary cardiomyopathies & 0.7652 & 0.2835 & 0.2666 & 0.2727 & 0.2608\\ 
Hyposmolality and/or hyponatremia & 0.7638 & 0.0104 & 0.0176 & 0.0090 & 0.4\\ 
Other and unspecified coagulation defects & 0.7635 & 0.1154 & 0.1086 & 0.0657 & 0.3125\\ 
Orthopaedic surgery & 0.7615 & 0.0389 & 0.0701 & 0.0384 & 0.4\\ 
Epilepsy & 0.7584 & 0.3188 & 0.3873 & 0.3282 & 0.4725\\ 
Mechanical complication of V-P shunt & 0.7580 & 0.0203 & 0.1 & 0.0833 & 0.125\\ 
Delayed milestones & 0.7564 & 0.3421 & 0.3944 & 0.3467 & 0.4574\\ 
Esophageal reflux & 0.7545 & 0.0585 & 0.1234 & 0.0833 & 0.2380\\ 
Croup syndrome & 0.7538 & 0.0403 & 0.0165 & 0.0083 & 0.7142\\ 
Heart disease & 0.7526 & 0.0426 & 0.0769 & 0.0666 & 0.0909\\ 
Subdural hemorrage following injury without open wound & 0.7477 & 0.0553 & 0.0810 & 0.0535 & 0.1666\\ 
Malignant neoplasm & 0.7431 & 0.0101 & 0.0152 & 0.0078 & 0.3333\\ 
History of surgery to major organs & 0.7429 & 0.0474 & 0.0454 & 0.0270 & 0.1428\\ 
Congenital central alveolar hypoventilation syndrome & 0.7400 & 0.0127 & 0.0095 & 0.0049 & 0.1428\\ 
Acute and subacute necrosis of the liver & 0.7383 & 0.1321 & 0.1904 & 0.1666 & 0.2222\\ 
Anemia & 0.7321 & 0.0388 & 0.0327 & 0.0173 & 0.2857\\ 
Dehydration & 0.7319 & 0.0360 & 0.0888 & 0.0588 & 0.1818\\ 
Unspecified disease of spinal cord & 0.7291 & 0.0614 & 0.0720 & 0.0421 & 0.25\\ 
Primary malignant neoplasm & 0.7274 & 0.0170 & 0.0270 & 0.0141 & 0.3\\ 
Urinary tract infection & 0.7259 & 0.0491 & 0.0941 & 0.0579 & 0.25\\ 
Malignancy of bone - no site specified & 0.7184 & 0.0180 & 0.0833 & 0.0487 & 0.2857\\ 
Drowning and non-fatal submersion & 0.7174 & 0.0146 & 0.0272 & 0.0142 & 0.2857\\ 
Observation of newborn or infant for supsected condition %not found
& 0.7169 & 0.0347 & 0.0683 & 0.04 & 0.2352\\ 
Insomnia with sleep apnea & 0.7108 & 0.2015 & 0.0961 & 0.0574 & 0.2941\\ 
Bone marrow transplant status & 0.7077 & 0.0770 & 0.0983 & 0.0588 & 0.3\\ 
Thrombocytopenia & 0.7060 & 0.0209 & 0.0512 & 0.0280 & 0.3\\ 
Unspecified intestinal obstruction & 0.7045 & 0.0495 & 0.0638 & 0.0379 & 0.2\\ 
Unspecified injury & 0.7020 & 0.0333 & 0.0 & 0.0 & 0.0\\ 
Unspecified disorder of intestine & 0.6961 & 0.0550 & 0.075 & 0.0468 & 0.1875\\ 
Blood in stool & 0.6908 & 0.0089 & 0.0245 & 0.0127 & 0.3333\\ 
Respiratory arrest & 0.6883 & 0.1622 & 0.1052 & 0.0833 & 0.1428\\ 
Malignant neoplasm & 0.6790 & 0.0590 & 0.0486 & 0.0254 & 0.5333\\ 
Panhypopituitarism & 0.6784 & 0.0146 & 0.0242 & 0.0127 & 0.25\\ 
Other complications of nervous sytem device & 0.6760 & 0.0132 & 0.0289 & 0.0153 & 0.25\\ 
Ostium secundum type atrial septal defect & 0.6750 & 0.0218 & 0.0437 & 0.0234 & 0.3333\\ 
Hereditary hemolytic anemia & 0.6733 & 0.0115 & 0.0262 & 0.0135 & 0.4285\\

\hline
\end{tabular} \hspace{-0.2in}
% \label{fig:single-label-total-results-2}
\label{tab:single-label-total-results-2}
\end{table*}
% \end{figure*}


% \begin{figure*}[ht]
\begin{table*}[ht]
\centering
\footnotesize
% \scriptsize
\begin{tabular}{|l|l|l|l|l|l|}
 \hline
 \multicolumn{6}{|c|}{(continued) Classifier Performance on Each Diagnostic Code Sorted by AUC} \\
 \hline
  Label & \textbf{AUC} & AUPRC & F1 & Precision & Recall \\
 \hline

Sickle-cell anemia & 0.6712 & 0.0093 & 0.0263 & 0.0134 & 0.6\\ 
Ventricular septal defect & 0.6580 & 0.0170 & 0.0444 & 0.025 & 0.2\\ 
Other specified cardiac dysrhytmia & 0.6554 & 0.0483 & 0.0168 & 0.0086 & 0.3333\\ 
Conditions due to anomaly of unspecified circumstance & 0.6537 & 0.0991 & 0.1637 & 0.1031 & 0.3965\\ 
Injury crushing, not otherwise specified & 0.6445 & 0.0085 & 0.0191 & 0.0098 & 0.4\\ 
Respiratory complications resulting from a procedure & 0.6385 & 0.0275 & 0.0291 & 0.0157 & 0.2\\ 
Hemophilus meningitis & 0.6240 & 0.0080 & 0.0135 & 0.0068 & 0.3333\\ 

Hematologic, other & 0.6078 & 0.0212 & 0.0394 & 0.0215 & 0.2352\\ 
Unspecified disorder of thyroid & 0.6068 & 0.0182 & 0.0151 & 0.0077 & 0.375\\ 
Disorders of the nervous system & 0.5847 & 0.0315 & 0.0553 & 0.0290 & 0.5652\\ 
Unspecified disorder of immune mechanism & 0.5658 & 0.0205 & 0.0377 & 0.0208 & 0.2\\ 
Unspecified disorder of metabolism & 0.5552 & 0.0313 & 0.0555 & 0.0454 & 0.0714\\ 
Gastrointestinal Surgery, other & 0.5412 & 0.0152 & 0.0241 & 0.0129 & 0.1875\\ 
Asthma, not otherwise specified & 0.5398 & 0.0168 & 0.0335 & 0.0175 & 0.4117\\ 
Tetralogy of fallot & 0.4325 & 0.0058 & 0.0082 & 0.0042 & 0.2857\\ 

\hline
\end{tabular} \hspace{-0.2in}
% \label{fig:single-label-total-results-3}
\label{tab:single-label-total-results-3}
\end{table*}
% \end{figure*}
